# Supplementary material for: Learning Equivariant Energy Based Models with Equivariant Stein Variational Gradient Descent
Source: arXiv:2106.07832 source file (2021-07-29)
Supplement: Supplementary file 1 [file soc.tex]

In this work, we proposed methods to incorporate prior information in the form of symmetries in probabilistic modelling. As such, we do not expect our work to lead to any negative risks to the society. However, the model and paradigms proposed in this paper for efficiently learning and training probabilistic models are quite general and can be used in many diverse fields like autonomous driving, drug-discovery, \etc and can thus cause both positive and negative impacts depending on how the model and approach is developed and deployed.
